# Supplementary material for: ScheduleStream: Temporal Planning with Samplers for GPU-Accelerated Multi-Arm Task and Motion Planning & Scheduling
Source: arXiv:2511.04758 source file (2026-05-28)
Supplement: Supplementary file 1 [file appendix.tex]

\subsection{Appendix}

\begin{thm} \label{thm:TBD}
CuStream plan existence is undecidable.
\begin{proof}
TBD
\end{proof}
\end{thm}

\begin{thm} \label{thm:TBD}
TBD is semi-complete.
\end{thm}

\subsection{Links}

\begin{itemize}
    \item \href{https://arxiv.org/abs/1802.08705}{PDDLStream}
    \item \href{https://www.overleaf.com/project/669ef0f5bbcc5f891bba3ad3}{William}
    \item \href{https://www.overleaf.com/project/6553ac4c975898cb37e805c1}{VLM-TAMP}
    \item \href{https://www.overleaf.com/project/6697508c126258f981103451}{Nishanth}
    \item \href{https://nvidia-my.sharepoint.com/:p:/r/personal/cgarrett_nvidia_com/Documents/Figures.pptx?d=wb51d3a6421524ab08f39c542eb51a4ba&csf=1&web=1&e=TYhz9A}{Figures}
    \item \url{https://www.overleaf.com/learn/latex/Font_sizes%2C_families%2C_and_styles}
    \item \url{https://www.overleaf.com/learn/latex/Mathematical_fonts}
    \item \url{https://artofproblemsolving.com/wiki/index.php/LaTeX:Symbols?srsltid=AfmBOoqPrAE5aXwlsR0CBIFx0cyMbQSVkVlR9UgxccdwIvDAFpTt-Ts0}
    \item \href{https://docs.google.com/presentation/d/1qxp3tP3TsSCIm3r4K4CMT_C-cO3ePBxUVmh71bBrpy0/edit}{Individual Updates}
    \item \href{https://nvidia-my.sharepoint.com/:p:/r/personal/cgarrett_nvidia_com/Documents/cuStream%
\end{itemize}

\subsection{Retime}

\begin{align*}
  \min_{\decision{p}, \decision{q} \in V}& \sum_{\pddl{Dist}(\decision{q}, \decision{q'}) \in C} |\decision{q'} - \decision{q}|_1 \\
 \suchthat & \decision{t}_{j+1} - \decision{t}_{j} \geq \constant{t}^0_{j+1} - \constant{t}^0_{j} \\
 & |\decision{s}_{i} - \decision{t}_{j}| \geq \epsilon, & \forall i,j.\;\proc{colliding}(x_i, y_j)
\end{align*}

\begin{itemize}
    \item Robots $R = \{r_1, ..., r_k\}$
    \item Path $[q_1^r, .., q_n^r]$ for robot $r \in R$
    \item Times $[\hat{t}_1^r, .., \hat{t}_n^r]$ for each path
\end{itemize}

\begin{align*}
  \min_{\decision{t}}& \max_{r \in R} \decision{t}_{n}^{r}  \\
 \suchthat & \decision{t}_{i+1}^{r} - \decision{t}_{i}^{r} \geq \hat{t}_{i+1}^r - \hat{t}_{i}^r, & \forall r \in R, i \in [n-1] \\
 & \decision{t}_{i+1}^{r} + \epsilon < \decision{t}_{j}^{r'}&\\
 &\kw{ or }\; \decision{t}_{j+1}^{r'} + \epsilon < \decision{t}_{i}^{r}, & \kw{when}\;\proc{colliding}(r, q_i^r, r', q_j^{r'})
\end{align*}

\subsection{Backup}

\noindent Constants:
\begin{footnotesize}
\begin{minted}{python}
# Continuous initial state
arm1 = "arm1"; arm2 = "arm2"
q1 = [...]; q2 = [...]

q1 = np.array([...]); q2 = np.array([...])
p1 = np.array([...]); p2 = np.array([...])
p1 = [[...], ...]
p1 = [[ . . . ],
      ...,
      [0 0 0 1]]

p1 = [[* * * *],
      ...,
      [0 0 0 1]]
p1, p2 = [[* * * *], [[* * * *],
          ...,           ...,
          [0 0 0 1]], [0 0 0 1]]
p1 = [[* * * *],...,[0 0 0 1]]

p1 = [[...], ..., [0 0 0 1]]
arm_confs = {arm1: q1, arm2: q1}
\end{minted}
\end{footnotesize}

\noindent Schedule:
\begin{footnotesize}
\begin{minted}{python}
schedule = [move(arm1, q1, "#q1")]

move1 = move(arm1,q1,"@t1","@q1")
pick1 = pick(arm1,"@q1","@g1",p1)
move2 = move(arm2,q2,"@t2","@q2")
pick2 = pick(arm2,"@q2","@g2",p2)

plan = [move1, pick1, move2, pick2]
schedule = [move1, pick1, move2, pick2]
of
plan = [|\class{Start}|(move_1), |\class{End}|(move_1), pick1, 
  |\class{Start}|(move2), |\class{End}|(move2), pick2]

plan = [move1.|\kwarg{start}|, move1.|\kwarg{start}|, pick1, 
  move2.|\kwarg{start}|, move2.|\kwarg{end}|, pick2]

plan = [|\class{Start}|(move1), |\class{End}|(move1), pick1, 
  |\class{Start}|(move1_2), |\class{End}|(move1_2),
  |\class{Start}|(move2), |\class{End}|(move2), pick2]

schedule = [
  |\class{TimedAction}|(move1,|\kwarg{start}|=0.,|\kwarg{end}|=1.),
  |\class{TimedAction}|(pick1,|\kwarg{start}|=1.,|\kwarg{end}|=1.),
  |\class{TimedAction}|(move2,|\kwarg{start}|=1.,|\kwarg{end}|=2.),
  |\class{TimedAction}|(pick2,|\kwarg{start}|=2.,|\kwarg{end}|=2.),
]
\end{minted}
\end{footnotesize}

\noindent Backup:
\begin{footnotesize}
\begin{minted}{python}
goal =  [At("arm1")==q1, At("arm2")==q2,
  Holding("arm1")=="obj1", Holding("arm2")=="obj2"]

Placement = |\class{Predicate}|("?obj ?p", 
  |\kwarg{cond}|=[Object("?obj")])

placements = |\class{Stream}|(Placement, |\kwarg{inps}|="?obj", |\kwarg{fn}|=...)

action = |\class{Action}|(|\kwarg{params}|="", |\kwarg{cond}|=[], |\kwarg{end}|=[])

action = |\class{DurativeAction}|(|\kwarg{params}|="", |\kwarg{start\_cond}|=[], 
  |\kwarg{start\_eff}|=[], |\kwarg{over\_cond}|=[], |\kwarg{end\_cond}|=[], |\kwarg{end\_eff}|=[],conditions
  |\kwarg{duration}|=1.0)

class Predicate(Function):
  ...
\end{minted}
\end{footnotesize}

\begin{algorithm}[bt]
    \caption{Temporal Planning}
    \label{alg:algorithm}
    \begin{algorithmic}[1]
    \begin{footnotesize}
        \Procedure{serialize}{$\tau$}
            \State $\pi \gets [\;]$
            \State $T \gets \{t \mid \langle t_1, a(x), t_2 \rangle \in \pi.\; t \in [t_1, t_2]\}$
            \For{$t \in \kw{sorted}(T)$}
                \For{$\langle t_1, a(x), t_2 \rangle \in \tau$}
                    \If{$t = t_1$}
                        \State $\pi \gets \pi + [a(x).\var{start}]$
                        \Comment{Apply effects}
                    \ElsIf{$t_1 < t < t_2$}
                        \State $\pi \gets \pi + [a(x).\var{over}]$
                    \ElsIf{$t = t_2$}
                        \State $\pi \gets \pi + [a(x).\var{end}]$
                    \EndIf
                \EndFor
            \EndFor
            \Comment{Extract stream plan directly}
            \State \Return $\pi$
        \EndProcedure
    \end{footnotesize}
    \end{algorithmic}
\end{algorithm}

\begin{algorithm}[bt]
    \caption{Temporal Planning}
    \label{alg:algorithm}
    \begin{algorithmic}[1]
    \begin{footnotesize}
        \Procedure{incremental}{${\cal I}, {\cal S}$}
            \State \Comment{Return stream plan here}
            \State \Comment{Do incremental here and return the stream plan}
        \EndProcedure

        \Procedure{algorithm}{${\cal I}, {\cal S}$}
            \State $I \gets \kw{copy}({\cal I})$; $\Psi \gets [\;]$
            \While{\True}
                \For{$s(x) \in \proc{instantiate}(I, {\cal S})$}
                    \State $y \gets \kw{next}(s.\var{fn}(x))$
                    \If{$s(x)(y) \notin \Psi$}
                        \State $\Psi \gets \Psi + [s(x)(y)]$
                        \For{$p \in s.\var{out\_cond}$}
                            \State $I[p(x,y)] \gets \kw{True}$
                        \EndFor
                    \EndIf
                \EndFor
            \EndWhile
        \State \Return $\Psi$
        \EndProcedure

        \Procedure{algorithm}{${\cal I}, {\cal G}, {\cal A}, {\cal S}$}
        \While{\True}
            \Comment{Subroutine that instantiates and applies}
            \State $S \gets \proc{lazy-streams}({\cal S})$
            \State $I \gets \proc{apply-streams}({\cal I}, S)$            
            \State $\tau \gets \proc{schedule}(I, {\cal G}, A)$
            \If{$\tau \neq \kw{None}$}
                \State $I \gets \{\langle f(x), y \rangle \in \proc{preimage}(\pi) \mid f(x) \notin I\}$
                \State $\psi \gets \proc{retrace-streams}(S, I)$
                \State $Q \gets Q + [\langle \psi, \tau \rangle]$
            \EndIf
            \For{$\langle \psi, \tau \rangle \in Q$}
                \State $\psi' \gets \proc{apply}(\psi)$ \Comment{Rollout}
                \If{$|\psi'| = |\psi|$}
                    \State \Return $\tau$
                \EndIf
                \State ${\cal I} \gets {}$
            \EndFor
        \EndWhile
        \EndProcedure
    \end{footnotesize}
    \end{algorithmic}
\end{algorithm}

\subsection{Batcher}

\begin{algorithm}[bt]
    \caption{Batch Constraint Sampling}
    \label{alg:algorithm}
    \begin{algorithmic}[1]
    \begin{footnotesize}
        \Procedure{process-batch-stream}{$\var{init}, \var{stream}, \var{inp}$}
            \State $\var{stream}.\attr{processed} \unioneq \{\var{inp}\}$
            \State $\var{stream}.\attr{batch} \unioneq \{\var{inp}\} $
            \If{$|\var{stream}.\attr{batch}| \geq \var{stream}.\attr{capacity}$}
                \For{$\langle \var{inp}', \var{out}' \rangle \in \var{stream}.\proc{call}(\var{stream}.\attr{batch})$}
                    \State $\var{stream}.\attr{pairs}[\var{inp}'] \unioneq \{\var{out}'\}$
                    \State $\var{binding} \gets \kw{zip}(\var{stream}.\pddlkw{inps} {+} \var{stream}.\pddlkw{outs}, \var{inp}' {+} \var{out}')$
                    \State $\var{init} \unioneq \proc{substitute}(\var{stream}.\pddlkw{certified}, \var{binding})$
                \EndFor
                \State $\var{stream}.\attr{batch} \gets \emptyset$
            \EndIf
        \EndProcedure
        \State
        \Procedure{batch-incremental}{$\var{init}, \var{goal}, \var{actions}, \var{streams}$}
        \While{\True}
            \State $\var{action-plan} \gets \proc{search}(\var{init}, \var{goal}, \var{actions})$
            \If{$\var{action-plan} \neq \None$}
                \State \Return \var{action-plan}
            \EndIf
            \For{$\var{stream} \in \var{streams}$}
                \For{$\var{inp} \in \proc{satisfying}(\var{init}, \var{stream}.\pddlkw{domain})$}
                    \State $\proc{process-batch-stream}(\var{init}, \var{stream}, \var{inp})$
                \EndFor
            \EndFor
        \EndWhile
        \EndProcedure
    \end{footnotesize}
    \end{algorithmic}
\end{algorithm}

\begin{equation*}
    \var{action\_plan} = [\var{action}_1(\var{param}_1), ..., \var{action}_n(\var{param}_n)]
\end{equation*}
\begin{equation*}
    \var{action\_plan} = [\var{action}_1(\var{?param}_1), ..., \var{action}_n(\var{?param}_n)]
\end{equation*}

\begin{equation*}
    \var{stream-plan} = [\var{stream}_1(\var{inp-param}_1){\to}\var{out-param}_1, ...]
\end{equation*}
\begin{equation*}
    \var{stream-plan} = [\var{stream}_1(\var{?inp}_1){\to}\var{?out}_1, ...]
\end{equation*}
\begin{equation*}
    \var{stream-plan} = [\var{stream}_1(\var{?inp}_1, \var{?out}_1), ...]
\end{equation*}
\begin{equation*}
    \var{stream-plan} = [\var{stream}_1[\var{?inp}_1, \var{?out}_1], ...]
\end{equation*}
\begin{equation*}
    \var{stream-plan} = [\var{stream}_1(\var{?inp}_1)(\var{?out}_1), ...]
\end{equation*}
\begin{equation*}
    \var{stream-plan} = [\var{stream}_1(\var{?i}_1){\to}\var{?o}_1, ...]
\end{equation*}
\begin{equation*}
    \var{stream-plan} = [\var{stream}_1(?i_1){\to}?o_1, ...]
\end{equation*}
\begin{equation*}
    \var{stream-plan} = [s_1(i_1){\to}o_1, ...]
\end{equation*}

\begin{algorithm}[bt]
    \caption{Batch Constraint Sampling}
    \label{alg:algorithm}
    \begin{algorithmic}[1]
    \begin{footnotesize}
        \Procedure{satisfy-plans}{$\var{init}, \var{queue}; T$}
            \State $t_0 \gets \proc{time}()$
            \While{$\kw{len}(\var{queue}) \neq 0 \;\kw{and}\; (\proc{time}() - t_0) \leq T$}
                \State $\langle \var{stream-plan}, \var{action-plan} \rangle \gets \proc{pop}(\var{queue})$
                \If{$\kw{len}(\var{stream-plan}) = 0$}
                    \State \Return \var{action-plan}
                \EndIf
                \State $(\var{stream}(\var{inp}) {\to} \var{?out}) \gets \var{stream-plan}[0]$
                \State $\proc{process-batch-stream}(\var{init}, \var{stream}, \var{inp})$
                \For{$\var{out} \in \var{stream}.\attr{pairs}[\var{inp}]$}
                    \State $\var{binding} \gets \kw{zip}(\var{?out}, \var{out})$
                    \State $\var{stream-plan}' \gets \proc{substitute}(\var{stream-plan}, \var{binding})[1{:}]$
                    \State $\var{action-plan}' \gets \proc{substitute}(\var{action-plan}, \var{binding})$
                    \State $\proc{push}(\var{queue}, \langle \var{stream-plan}', \var{action-plan}' \rangle)$
                \EndFor
                \State $\proc{push}(\var{queue}, \langle \var{stream-plan}, \var{action-plan} \rangle)$
            \EndWhile
            \State \Return \None
        \EndProcedure
        \State
        \Procedure{optimistic-streams}{$\var{init}, \var{streams}$}
            \State $\var{init}^* \gets \{\var{atom}: \kw{None} \;\kw{for}\; \var{atom} \in \var{init}\}$
            \While{\True}
            \State $\var{size} \gets |\var{init}^*|$
            \For{$\var{s} \in \var{streams}$}
                \For{$\var{inp}^* \in \proc{satisfying}(\var{init}^*, \var{s}.\pddlkw{domain})$}
                    \If{$\var{inp}^* \notin \var{s}.\attr{processed}$}
                        \State $\var{out}^* \gets \proc{OptimisticOutput}(\var{s}, \var{inp}^*)$                    
                        \State $\var{binding}^* \gets \kw{zip}(\var{s}.\pddlkw{inps} {+} \var{s}.\pddlkw{outs}, \var{inp}^* {+} \var{out}^*)$
                        \For{$\var{atom}^* \in \proc{substitute}(\var{s}.\pddlkw{cert}, \var{binding}^*)$}
                            \State $\var{init}^*[\var{atom}^*] \gets (\var{s}(\var{inp}^*) {\to} \var{out}^*)$
                        \EndFor
                    \EndIf
                \EndFor
            \EndFor
            \If{$|\var{init}^*| = \var{size}$}
                \State \Return $\var{init}^*$
            \EndIf
            \EndWhile
        \EndProcedure
        \State
        \Procedure{batch-deferred}{$\var{init}, \var{goal}, \var{actions}, \var{streams}$}
        \State $\var{queue} \gets [\;]$
        \While{\True}
            \State $\var{init}^* \gets \proc{optimistic-streams}(\var{init}, \var{streams})$
            \State $\var{action-plan}^* \gets \proc{search}(\var{init}^*, \var{goal}, \var{actions})$
            \If{$\var{action-plan}^* \neq \None$}
                \State $\var{stream-plan}^* \gets \proc{retrace-streams}(\var{init}^*, \var{action-plan}^*)$ %
                \State $\proc{push}(\var{queue}, \langle \var{stream-plan}^*, \var{action-plan}^* \rangle)$ 
            \EndIf
            \State $\var{action-plan} \gets \proc{process-plans}(\var{init}, \var{queue})$
            \If{$\var{action-plan} \neq \None$}
                \State \Return $\var{action-plan}$
            \EndIf            
        \EndWhile
        \EndProcedure
    \end{footnotesize}
    \end{algorithmic}
\end{algorithm}

\subsection{Ideas}

Differences from GPU-TAMP
\begin{itemize}
    \item Representational contribution
    \item Multiple algorithms
    \item Backtrack over skeletons
    \item Modular computation graph
    \item Share samplers among task plans
    \item Sphere-mesh collision checking
    \item Optimization within samplers
    \item CuRobo software
\end{itemize}

Ideas:
\begin{itemize}
    \item Differentiable constraints and projection
    \item Compositional
    \item Backtracking across plan skeletons
    \item Multiple plan skeleton types
    \item Multiple algorithms
    \item Navigation
    \item Batching on different input types
    \item Motion planning to goal poses
    \item Parallel trajectory optimization
    \item Optimization
    \item Static vs movable
    \item Project onto constraint manifold
    \item Figure with multiple plan skeletons (directly place vs move)
    \item Generic Figures PowerPoint
    \item Gradient free
    \item Neighborhood of solutions for some samplers
    \item Distance function on samples (helps with Stein as well)
    \item React to online observations (decompose move into an MPC and full traj)
    \item Stein
    \item Incremental and focused algorithm 
    \item cuStream, GPU-Stream, cuTAMP, GPU-TAMP, cuPlan, NVPlan, ScheduleStream, TemporalStream, PyStream, PyPlan, FunctionalStream, MultiStream, DurativeStream, BatchStream
    \item Task and Motion Scheduling (TAMS)
    \item Task and Motion Planning and Scheduling (TAMPAS)
    \item Task and Motion Planning \& Scheduling (TAMPS)
\end{itemize}

Advanced Algorithms
\begin{itemize}
    \item Shared optimistic outputs (instead of unique)
    \item Merge deferred and incremental
    \item Anytime optimization
    \item Selectively return values
\end{itemize}

Random
\begin{itemize}
    \item Batchers that require common args (collisions possibly)
    \item Assume all are batchers or separate batcher vs stream
    \item Target batch size
    \item Use inputs and outputs instead of $x$ and $y$
    \item Write the algorithms and notation more clearly the second time
    \item Describe the value return phase with best bindings
    \item Ordering with bindings
    \item Reference my thesis and describe other algorithms there
    \item Detect when no upstream values
    \item Eager batcher instantiation
    \item Anytime mode
    \item Prune when dominated
    \item Upstream values on the plan
    \item Reuse across plans and time
    \item Optimization within streams
    \item Use textt or textsc instead of math
    \item Bias away from initial placements
    \item Sample from the set of motion solutions once one is identified
    \item Forbid version of the algorithm
    \item Unify adaptive and forbid
    \item Should we call these streams? Yes, streams have state.
    \item Explain extensions
    \item Use for constraint satisfaction or sampling
\end{itemize}

\subsection{Experiments}

Objectives:
\begin{itemize}
    \item Beat prior work
    \item Complicated examples
    \item Humanoid
    \item More than 2 arms
    \item Need TAMP
\end{itemize}

Approaches:
\begin{itemize}
    \item Incremental vs focused?
    \item Batch vs serial operations
    \item Batcher vs normal
    \item PyBullet vs curobo
    \item Sequential adaptive~\cite{garrett2020PDDLStream}
    \item Post processing
    \item Robot scaling for same task
\end{itemize}

Metrics:
\begin{itemize}
    \item Time to first solution
    \item First solution makespan
    \item Convergence time
    \item Convergence makespan
    \item Compare makespan across approaches?
\end{itemize}

Simulated:
\begin{itemize}
    \item Dual arms (Panda or SO-100)
    \item Multiple arms (Panda or SO-100)
    \item G1 or GR1
    \item Torso usage
    \item Mobile manipulation
    \item Handover
    \item Constrained motion
    \item Articulated objects (drawer)
    \item TAMP examples
    \item Tools
    \item Multiple goals
    \item Scale number of robots
\end{itemize}

Real:
\begin{itemize}
    \item Rummy Robotiq
    \item Rummy Dexterous
    \item SO-100
\end{itemize}

\begin{figure}[t]
    \centering
    \includegraphics[width=0.5\textwidth]{figures/wild-batching-reverse.png}
    \caption{\small{\textbf{TBD.} TBD.}}
    \label{fig:TBD}
    \vspace{-1em}
\end{figure}

\subsection{Abstract}

Many autonomous systems, such as robot manipulators, must make mixed discrete-continuous decisions in order to accomplish their tasks. 
However, this hybrid reasoning, for example, during robot task and motion planning, can be computationally taxing due to the large space of possible yet unproductive discrete plan types and continuous plan parameter values.
We seek to provide a planning framework that can flexibly model and efficiently solve these problems.
To that end, we propose a domain-independent action language for hybrid planning using blackbox batched sampling operations.
Batched samplers can be parallelized, for example using GPU-acceleration, in order to generate constraint-satisfying values simultaneously and more quickly than generating them serially.
Additionally, we introduce novel algorithms that efficiently make use of batched samplers when considering multiple candidate plans and multiple invocations in a plan simultaneously.
Our experiments show that GPU-accelerated batched sampling results in improved algorithmic performance in simulation.
We demonstrate our approach on several real-world manipulation tasks.
